# Supplementary material for: Using an LLM to Help With Code Understanding
Source: arXiv:2307.08177 source file (2024-01-16)
Supplement: Supplementary file 1 [file appendix.tex]

\onecolumn
% \newpage
% \appendices

\lstset {
    language=python,                  % language code
    basicstyle=\footnotesize,      % font size
    numbers=none,                  % where to put line numbers
    numberstyle=\footnotesize,     % numbers size
    numbersep=5pt,                 % how far the line numbers are from the code
    showspaces=false,                          % show spaces (with underscores)
    showstringspaces=false,            % underline spaces within strings
    showtabs=false,                            % show tabs using underscores
    frame=single,                  % adds a frame around the code
    tabsize=4,                     % default tabsize
    breaklines=true,                  % automatic line breaking
    columns=fullflexible,
    breakautoindent=false,
    xleftmargin=0pt,
    xrightmargin=0pt,
    breakindent=0pt,
    resetmargins=true
}

\begin{table*}[!ht]
\caption{An example code context and the information that can be provided by our tool given the code.}
\begin{tabular}{p{0.1\linewidth}  p{0.85\linewidth}}
\toprule
\multicolumn{2}{c}{\textbf{Code Context}}        \\ \midrule
Selected code &
\noindent
\begin{minipage}[t]{\linewidth}
\vspace{-.25cm}
\begin{lstlisting}[language=python]
bunny = o3d.data.BunnyMesh()
bunny_mesh = o3d.io.read_triangle_mesh(bunny.path)
bunny_mesh.compute_vertex_normals()
bunny_mesh.transform([[1, 0, 0, 0], [0, -1, 0, 0], [0, 0, -1, 0], [0, 0, 0, -1]])
bunny_mesh.translate([2.5, 2.1, 1.2])
\end{lstlisting}
\vspace{-.15cm}
\end{minipage}
\\ \midrule
\multicolumn{2}{c}{\textbf{One-click Prompting}} \\ \midrule
Overview                   & This code loads a mesh of a bunny, computes its vertex normals, applies a transformation matrix to invert and translate it.           \\ \midrule
API                        &  
- The first line of code loads the bunny mesh from the open3d data module.\newline
- The second line reads the triangle mesh of the bunny from the file path.\newline
- The third line computes the vertex normals of the bunny mesh, which are used to determine the orientation of each vertex with respect to the surface of the mesh.\newline
- The fourth line applies a transformation matrix to the bunny mesh using the \path{transform} function. The matrix used in this case is a 4x4 matrix that performs a reflection along the x-axis, followed by a reflection along the y-axis, and finally a reflection along the z-axis. This effectively inverts the bunny mesh.\newline
- The fifth line applies a translation to the bunny mesh using the \path{translate} function. The translation vector used in this case is [2.5, 2.1, 1.2], which moves the bunny mesh 2.5 units along the x-axis, 2.1 units along the y-axis, and 1.2 units along the z-axis.        \\ \midrule
Concept                    & 
Here are 3 domain concepts that might be useful to know.\newline
- Mesh: A mesh is a collection of vertices, edges, and faces that define the shape of a 3D object. In open3d, a mesh is represented by a TriangleMesh object.\newline
- Vertex Normals: Vertex normals are vectors that are perpendicular to the surface of a mesh at each vertex. They are used to determine how light interacts with the surface of the mesh.\newline
- Transformation Matrix: A transformation matrix is a mathematical matrix that is used to transform a 3D object. In open3d, a transformation matrix is represented by a 4x4 matrix, where the first three columns represent the rotation and scaling of the object, and the last column represents the translation.\\ \midrule
Usage                       & Here is a open3d code example. \newline
\begin{minipage}[t]{\linewidth}
\vspace{-.15cm}
\begin{lstlisting}[language=python]
import open3d as o3d

# Load a mesh of a bunny
bunny = o3d.data.BunnyMesh()
bunny_mesh = o3d.io.read_triangle_mesh(bunny.path)

# Compute vertex normals
bunny_mesh.compute_vertex_normals()

# Apply transformation matrix to invert and translate the bunny mesh
transformation_matrix = [[1, 0, 0, 0], [0, -1, 0, 0], [0, 0, -1, 0], [0, 0, 0, -1]]
bunny_mesh.transform(transformation_matrix)
bunny_mesh.translate([2.5, 2.1, 1.2])

# Visualize the transformed bunny mesh
o3d.visualization.draw_geometries([bunny_mesh])
\end{lstlisting}
\end{minipage}
This code loads a mesh of a bunny, computes its vertex normals, applies a transformation matrix to invert and translate it, and finally visualizes the transformed bunny mesh.
\\ \midrule
\multicolumn{2}{c}{\textbf{Query Prompting}}     \\ \midrule
Query                      & How can I move bunny to sit upright?           \\ \midrule
Response                   & 
In this code, the bunny mesh is transformed using a 4x4 transformation matrix. To move the bunny to sit upright, you can apply a rotation transformation to the mesh. For example, you can rotate the mesh 90 degrees around the x-axis by using the following transformation matrix:
\newline
\begin{minipage}[t]{\linewidth}
\vspace{-.15cm}
\begin{lstlisting}[language=python]
[[1, 0, 0, 0],
 [0, 0, 1, 0],
 [0, -1, 0, 0],
 [0, 0, 0, 1]]
 \end{lstlisting}
\end{minipage}

You can apply this transformation to the bunny mesh using the \path{transform} method:\newline
\begin{minipage}[t]{\linewidth}
\vspace{-.15cm}
\begin{lstlisting}[language=python]
bunny_mesh.transform([[1, 0, 0, 0], [0, 0, 1, 0], [0, -1, 0, 0], [0, 0, 0, 1]])
\end{lstlisting}
\end{minipage}\newline
This will rotate the bunny mesh 90 degrees around the x-axis, making it sit upright.
\\ \bottomrule
\end{tabular}
\end{table*}

\begin{table}[htpb]
\caption{Completion time (s) of each subtask.}
\begin{tabular}{@{}lrrrrrr@{}}
\toprule
\multirow{2}{*}{} & \multicolumn{2}{c}{\textbf{All}} & \multicolumn{2}{c}{\textbf{Professionals}} & \multicolumn{2}{c}{\textbf{Students} }\\ 
& \multicolumn{1}{c}{\tool}    & Search   & \multicolumn{1}{c}{\tool}         & Search        & \multicolumn{1}{c}{\tool}      & Search      \\ \midrule [0.3pt] \midrule
                  % & \multicolumn{1}{c}{(32)}         & \multicolumn{1}{c}{(32)}       & \multicolumn{1}{c}{(9)}                 & \multicolumn{1}{c}{(7)}             & \multicolumn{1}{c}{(7)}              & \multicolumn{1}{c}{(9)}           \\\midrule
% \# Participants   & 16 & 16 & 9 & 7 & 7 & 9 \\ \midrule
Bokeh-1           & 193.75         & 202.8     &  244.86             & 239.25          & 122.20           & 178.50        \\
Bokeh-2           & 352.47         & 321.63     & 263.00              & 429.50          & 486.67           & 213.75        \\
Bokeh-3           & 610.86         & 764.20     & 634.75              & 723.83          & 579.00           & 791.11        \\
Bokeh-4           & 295.63         & 156.11     & 351.75              & 127.80          & 239.50           & 191.50        \\ \midrule [0.3pt] \midrule
                  % & \multicolumn{1}{c}{(32)}         & \multicolumn{1}{c}{(32)}       & \multicolumn{1}{c}{(7)}                 & \multicolumn{1}{c}{(9)}             & \multicolumn{1}{c}{(9)}              & \multicolumn{1}{c}{(7)}           \\\midrule
% \# Participants   & 16 & 16 & 7 & 9 & 9 & 7 \\ \midrule
Open3d-1          & 483.47         & 503.80     & 458.38              & 663.00          & 505.78           & 265.00        \\
Open3d-2          & 371.53         & 603.80     & 307.29              & 474.38          & 427.75           & 751.71        \\
Open3d-3          & 408.83         & 326.67     & 454.67              & 267.67          & 363.00           & 444.67        \\
Open3d-4          & 329.00         & 260.00     & 351.33              & 520.00          & 262.00           & -           \\ \bottomrule
\end{tabular}
\end{table}

\begin{table}[htpb]
\caption{Completion rates of each subtask.}
\begin{tabular}{@{}lrrrrrr@{}}
\toprule
\multirow{2}{*}{} & \multicolumn{2}{c}{\textbf{All}} & \multicolumn{2}{c}{\textbf{Professionals}} & \multicolumn{2}{c}{\textbf{Students} }\\ 
& \multicolumn{1}{c}{\tool}    & Search   & \multicolumn{1}{c}{\tool}         & Search        & \multicolumn{1}{c}{\tool}      & Search      \\ \midrule [0.3pt] \midrule
                  % & \multicolumn{1}{c}{(32)}         & \multicolumn{1}{c}{(32)}       & \multicolumn{1}{c}{(9)}                 & \multicolumn{1}{c}{(7)}             & \multicolumn{1}{c}{(7)}              & \multicolumn{1}{c}{(9)}           \\\midrule
% \# Participants   & 16 & 16 & 9 & 7 & 7 & 9 \\ \midrule
Bokeh-1           & 1.00         & 1.00     & 1.00              & 1.00          & 1.00           & 1.00        \\
Bokeh-2           & 0.88         & 0.81     & 0.89              & 0.71          & 0.86           & 0.89        \\
Bokeh-3           & 0.38         & 0.38     & 0.44              & 0.43          & 0.29           & 0.33        \\
Bokeh-4           & 0.25         & 0.56     & 0.22              & 0.57          & 0.29           & 0.56        \\ \midrule [0.3pt] \midrule
                  % & \multicolumn{1}{c}{(32)}         & \multicolumn{1}{c}{(32)}       & \multicolumn{1}{c}{(7)}                 & \multicolumn{1}{c}{(9)}             & \multicolumn{1}{c}{(9)}              & \multicolumn{1}{c}{(7)}           \\\midrule
% \# Participants   & 16 & 16 & 7 & 9 & 9 & 7 \\ \midrule
Open3d-1          & 0.81         & 0.69     & 1.00              & 0.67          & 0.67           & 0.71        \\
Open3d-2          & 0.81         & 0.50     & 1.00              & 0.44          & 0.67           & 0.57        \\
Open3d-3          & 0.50         & 0.13     & 0.57              & 0.11          & 0.44           & 0.14        \\
Open3d-4          & 0.06         & 0.06     & 0.00                 & 0.11          & 0.11           & -         \\ \bottomrule
\end{tabular}
\end{table}

\begin{table}[htpb]
\caption{Understanding scores.}
\begin{tabular}{@{}lrrrrrr@{}}
\toprule
\multirow{2}{*}{} & \multicolumn{2}{c}{\textbf{All}} & \multicolumn{2}{c}{\textbf{Professionals}} & \multicolumn{2}{c}{\textbf{Students} }\\ 
& \multicolumn{1}{c}{\tool}    & Search   & \multicolumn{1}{c}{\tool}         & Search        & \multicolumn{1}{c}{\tool}      & Search      \\ \midrule [0.3pt] \midrule
                  % & \multicolumn{1}{c}{(32)}         & \multicolumn{1}{c}{(32)}       & \multicolumn{1}{c}{(9)}                 & \multicolumn{1}{c}{(7)}             & \multicolumn{1}{c}{(7)}              & \multicolumn{1}{c}{(9)}           \\\midrule
% \# Participants   & 16 & 16 & 9 & 7 & 7 & 9 \\ \midrule
Bokeh           & 1.19         & 1.31     & 1.33              & 1.43          & 1.00           & 1.22        \\ \midrule [0.3pt] \midrule
% \# Participants   & 16 & 16 & 7 & 9 & 9 & 7 \\ \midrule
Open3d          & 0.75         & 0.125     & 1.43              & 0.11          & 0.22           & 1.14        \\ \bottomrule
\end{tabular}
\end{table}

\begin{table}[htpb]
\small
\setlength{\tabcolsep}{4pt} 
\caption{Participants' feedback codebook. The codes discussed in the paper are underlined. Initially, two authors separately performed open coding on the same set of 8 responses (25\% of the entire data), and convened to discuss and merge the codes into a shared codebook.
The first author coded the rest of the responses and discussed with the rest of the authors whenever new codes needed to be added.}
\centering
% \begin{tabular}{p{0.08\textwidth}  p{0.25\textwidth} p{0.45\textwidth}}
\begin{tabular}{C{1.4cm}L{6.5cm}L{9.5cm}}
% \begin{tabularx}{\columnwidth}{L*{3}}
% \begin{tabular}{cll}
\toprule
 & \textbf{Code \& Description} & \textbf{Representative Quote} \\ \midrule                                                                    
& \textbf{[Reduced initial apprehension effort]} \newline
The tool helps identify what to look for.                     & 
% The generated explanation of the code really helped to reduce the initial apprehensions one has while working with a new code base. 
I was able to identify which sections of the code I need to modify much faster with the extension, even though I have no prior knowledge of 3D rendering. (P25) \\ \cmidrule{2-3} 
& \underline{\textbf{[Context-adjusted response]}} \newline The tool provides code or explanation that is tailored to the user code.                          
& Biggest difference using AI-based VS code extension is that the given solutions are specific to the code you are actually writing, whereas searching the web are usually more general solutions. (P32) \\ \cmidrule{2-3} 
& \textbf{[Amazement]} \newline General positive reaction for a new tool.  & I was surprised how good the explanations were, how tailored it was to the code, how easily it could make the changes that were required, 
% and how fitting the answers were.
(P12)\\ \cmidrule{2-3} 
& \textbf{[Interactivity]} \newline Interactivity of the tool helps probing LLM. & The AI-based extension can be more interactive than search engines by maintaining conversation history. (P5) \\ \cmidrule{2-3} 
& \underline{\textbf{[Less context switching]}} \newline The tool does not break the workflow and saves clicks as it is integrated in IDE.   & … I can accomplish everything within the IDE without having to context switch to other resources (P3)  \\ \cmidrule{2-3} 
& \textbf{[Sufficient library details]} \newline The tool provides sufficient library information. & AI-based code extension was useful in a sense that it could also provide some details on concept, which could definitely help one to better tackle the task. (P28)  \\ \cmidrule{2-3} 
& \underline{\textbf{[Context incorporation]}} \newline The tool provides the ability to easily incorporate the context & 
(LLM-based AI programming tool is) better (than search engines). Since I don't need to come up with the good searching words (P20) 
% I like that it's able to use the context of the code that I'm actually editing, so hopefully it should be able to answer my questions without me explicitly telling it everything I'm doing.  (P2)  
\\ \cmidrule{2-3} 
& \textbf{[Varying granularity]} \newline The tool provides the ability to prompt about code at different granularity  & Being able to change your level of insight was helpful (highlighting certain portions of code vs overall knowledge about the entire program (P15)  \\ \cmidrule{2-3} 
\multirow{-27}{*}{\textbf{Pros}}           
& \underline{\textbf{[Less information foraging]}} \newline The tool reduces the need for information foraging.  & The main advantage for me is in circumventing the reading of the documentation. Official documentation is often lacking examples or short and concise explanations. For this reason, I often resort to stack overflow, in search of usage examples. 
% The ability to highlight an unknown line of code and know immediately what it does can therefore be incredibly valuable. 
(P24)\\ \midrule
& \textbf{[Required knowledge level for tool utility]} \newline The tool is more useful when a user \underline{has / does not have} existing knowledge.  & It would be more useful when I learn a new library/PL. (P13) \newline AI based are more helpful when you already know what the outcome should be (P11) \\ \cmidrule{2-3} 
& \underline{\textbf{[User interface]}} \newline The user interface of the tool is \underline{usable / can be improved}.  &I liked the different buttons for different types of information so I didn't have to read a lot of text to find what I was looking for (P7) \newline A simpler view would be nice, I felt like there were too many features which could get some time to get used to. (P8)  \\ \cmidrule{2-3} 
\multirow{-11}{*}{\textbf{Mixed}} & \textbf{[Pull-based interaction]} \newline Pull-based interaction is \underline{useful / not useful}.  & 
% When it comes to small snippets of code, 
GitHub Copilot's autocomplete is faster as it automatically suggests what I'm supposed to type next. But I can't actually ask co-pilot follow up questions, which I can do in the ai-based vs code extension, and that makes it really helpful. (P1)  \\ \midrule
& \textbf{[No correctness guarantee]} \newline The lack of trust and correctness guarantee of the outputs.  & 
% Using the AI-based extension, we can get a response much faster
... but there's always an underlying doubt in our mind regarding whether the information provided is 100\% factual or useful. (P24)  \\ \cmidrule{2-3} 
& \underline{\textbf{[Prompt dependency]}} \newline 
% The ability to prompt the model directly is useful to have / not necessary.  
The quality of the LLM-generated information depends on well-crafted prompts.
& 
AI-based VS code extension was not able to give me the code that I was looking for, so it took up all my time (which I got very annoyed about). I think I just didn't word the question well. (P28) \\ \cmidrule{2-3}
\multirow{-8}{*}{\textbf{Cons}}           
& \textbf{[Information diversity]} \newline The tool provides less diverse information compared to search engine results.  & Stack overflow provides user historical comments and may be important for different approaches to the same problem. (P30)  \\ \bottomrule
\end{tabular}
\end{table}

\begin{table}[htpb]
\small
\setlength{\tabcolsep}{4pt} 
\centering
\begin{tabular}{C{1.4cm}L{6.5cm}L{9.5cm}}
\toprule
 & \textbf{Code \& Description} & \textbf{Representative Quote} \\ \midrule   
& \underline{\textbf{[Other resources]}} \newline Add (links to) other relevant resources like documentation and Stack Overflow posts.  & I hope it can be combined with a documentation of the library, which makes it more accurate when providing descriptions of a method. (P21)  \\ \cmidrule{2-3} 
& \textbf{[LLM debugging capability]} \newline Ability to debug or auto-repair LLM outputs.  & The ability to interactively debug incorrect AI-proposed solutions would be helpful. (P5)  \\ \cmidrule{2-3} 
& [\textbf{LLM performance}] \newline Use more powerful and faster underlying LLM. & They were both quite verbose even when a single line would've sufficed. (P24) \\ \cmidrule{2-3} 
\multirow{-12}{*}{\textbf{Suggestions}}    
& \textbf{[Explainability]} \newline Add ability to provide the rationale behind the outputs.  & I think it may be better if we could understand the why aspect of the code. (P10) \\ \bottomrule
\end{tabular}
\end{table}

% \begin{figure}
%     \centering
%     \includegraphics[width=0.7\linewidth]{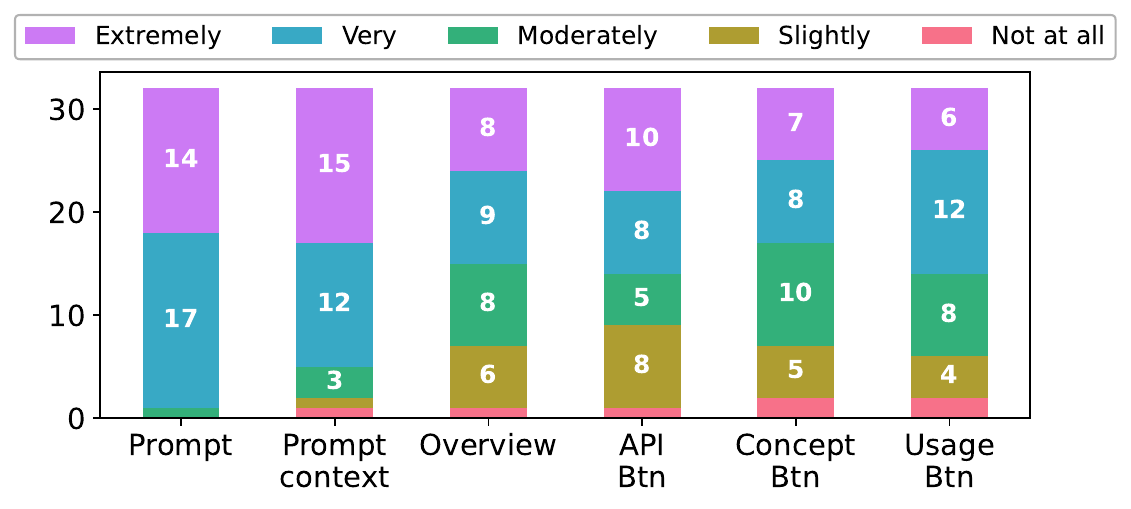}
%     \caption{Participants' report on the importance of \tool features.}
%     \label{fig:feature_importance}
% \end{figure}

% \begin{figure*}[htpb]
\begin{figure}[htpb]
% \begin{minipage}[tl]{.3\textwidth}
    \centering
    \includegraphics[width=0.3\textwidth]{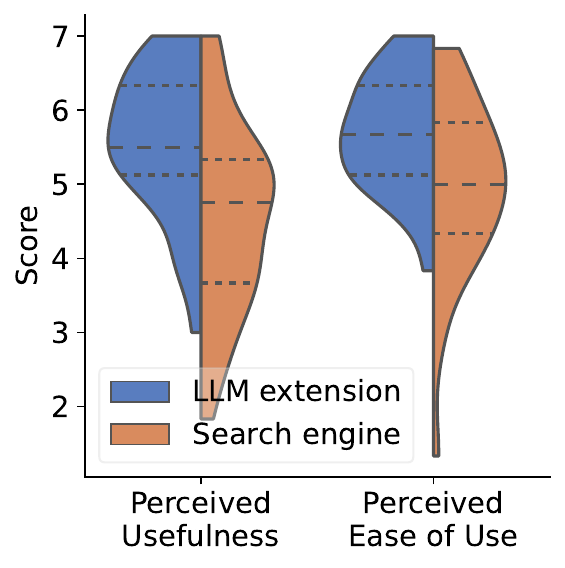}
    \caption{Response to TAM items}
    \label{fig:tam}
\end{figure}

\begin{figure}[htpb]
% \begin{minipage}[tr]{.65\textwidth}
    \centering
    \vspace{0pt}
    \includegraphics[width=0.7\textwidth]{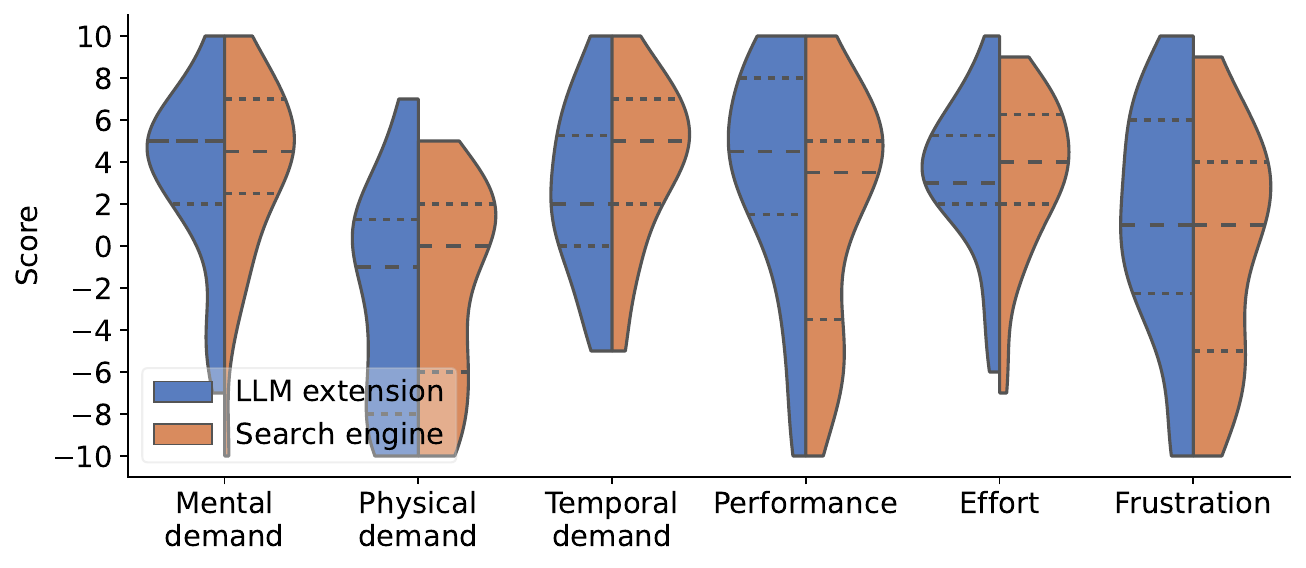}
    \caption{Response to NASA TLX items}
    \label{fig:tlx}
% \end{minipage}
\end{figure}
